# Supplementary material for: Phonon-assisted diffusion in bcc phase of titanium and zirconium from first-principles
Source: arXiv:1910.05806 source file (2020-04-24)
Supplement: Supplementary file 1 [file kadkhodaei_supplemenral_arxiv.pdf]

***Supplemental Materials:***

**Phonon-assisted diffusion in bcc phase of titanium and zirconium  
from first-principles**

Sara Kadkhodaei\* and Ali Davariashtiyani

*University of Illinois at Chicago, Chicago, Illinois, USA*

(Dated: April 24, 2020)

---

\* To whom correspondence should be addressed; Email: [sarakad@uic.edu](mailto:sarakad@uic.edu)

## SI. CALCULATION OF TEMPERATURE-DEPENDENT PHONON DISPERSION AND DENSITY OF STATES

Within the harmonic approximation, the Hamiltonian of the system is described as the following, for a system of  $N$  particles

$$\mathcal{H} = \frac{1}{2} \sum_{i=1}^N \sum_{\alpha=1}^3 \left[ \sqrt{M_i} \dot{u}_{i\alpha} \right]^2 + \frac{1}{2} \sum_{i,j}^N \sum_{\alpha,\beta}^3 \sqrt{M_i} u_{i\alpha} \frac{\Phi_{i,j}^{\alpha,\beta}}{\sqrt{M_i M_j}} \sqrt{M_j} u_{j\beta} \quad (1)$$

where  $u_{i\alpha}$  is the displacement of atom  $i$  in the  $\alpha$  direction,  $M_i$  is the mass of atom  $i$  and  $\Phi$  is the  $3N \times 3N$  force-constant matrix. Diagonalizing the dynamical matrix  $\frac{\Phi_{i,j}^{\alpha,\beta}}{\sqrt{M_i M_j}}$  as

$$\sum_j^N \sum_{\beta}^3 \frac{\Phi_{i,j}^{\alpha,\beta}}{\sqrt{M_i M_j}} \epsilon_{\mu}^{j\beta} = \omega_{\mu}^2 \epsilon_{\mu}^{i\alpha} \quad (2)$$

results in obtaining the phonon frequencies,  $\omega_{\mu}$  and eigenvectors,  $\epsilon_{\mu}^{i\alpha}$ . If the force-constant matrix is not positive-definite, some of the frequencies have imaginary values. We utilize two variations of the self-consistent harmonic approximation (SCHA) [1–5], which describes a harmonic model that minimizes the free energy rather than potential energy, which are significantly different in cases where harmonic phonon instabilities exist.

The self-consistent *ab initio* lattice dynamics (SCAILD) method [1–3] calculates atomic displacements based on an initial guess for phonon frequencies and accordingly updates the forces from first-principles calculation. A new set of phonon frequencies are obtained from the Fourier transformation of the updated atomic forces. This self-consistent process is performed until the difference in the vibrational free energy is converged to  $10^{-5}$  eV, as shown in Fig. S1(b). Fig. S1(a) illustrates this iterative process performed on a  $6 \times 6 \times 6$  supercell of bcc Ti including 216 atoms. The darkest dispersion curve in Fig. S1(a) corresponds to the harmonic phonon dispersion or zero-temperature phonon dispersion. The evolution of the phonon dispersion that includes the temperature-induced anharmonic effects is presented by smoothly varying the color of the curve from green to yellow (i.e., darkest to lightest). The converged phonon dispersion indicates no negative (imaginary) phonon frequencies as expected due to the dynamical stabilization of the phase at high enough temperature.

In the temperature-dependent effective potential (TDEP) method [4, 5], the temperature-dependent force-constant,  $\tilde{\Phi}(T)$ , is obtained by minimizing the difference between *ab initio* molecular dynamics (AIMD) forces and forces described in the harmonic approximation

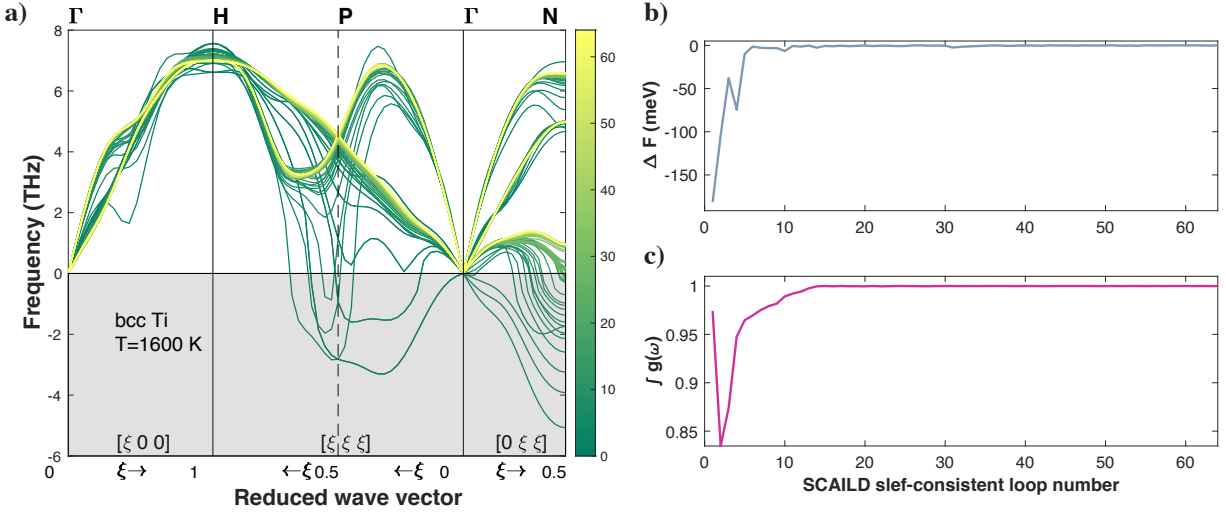

FIG. S1. a) Iterative evolution of anharmonic phonon dispersion for bcc Ti at 1600 K, obtained from the SCAILD method. The color bar indicates the iterative steps. The darkest color indicates the initial step, where the phonon dispersion is calculated using the harmonic approximation, as opposed to the lightest color which indicates the final step. b) The vibrational free energy difference,  $\Delta F$ , between consecutive SCAILD steps. The iterative steps are performed until  $\Delta F$  is smaller than  $10^{-5}$  eV. c) The evolution of the integral of phonon density of states along the SCAILD iterative steps.

according to the following equation,

$$\min \frac{1}{N_t} \sum_{t=1}^{N_t} \|f_t^{AIMD} - f_t^H\| = \min_{\tilde{\Phi}(T)} \frac{1}{N_t} \sum_{t=1}^{N_t} \|f_t^{AIMD} - \tilde{\Phi}(T)u_t^{AIMD}\| \quad (3)$$

where  $\{f_t^{AIMD}, u_t^{AIMD}\}$  are the set of AIMD forces and displacements obtained from the AIMD trajectory of length  $N_t$ . We performed AIMD simulations for each temperature using an  $NVT$  ensemble under the Nose–Hoover thermostat formalism [6–10]. The temperature-dependent force constant tensor is obtained by least square fitting of AIMD forces and displacements to a harmonic model according to Eq. 3 using our in-house code. The AIMD forces and displacement are captured every 0.01 ps in a trajectory of 35 ps, after thermalization of the system for 1 ps (for details on the burning and decay time see the next section). Fig. S2 illustrates the anharmonic phonon dispersion and density of states for bcc Ti in the range of 1300 to 1600 K, obtained from temperature-dependent force constant tensors using the Phonopy code [11]. There is a slight difference between the dispersion curves obtained

from SCAILD and TDEP, which stems from the different approaches taken in these methods to optimize the effective harmonic model to the Hamiltonian in Eq. 1. In SCAILD, the iterative steps are taken in the frequency-polarization space (the Fourier transformed of time-space pair) by assuming that the polarization vectors are constant and only phonon frequencies are optimized (see Eq. 2). However, in TDEP the polarization vectors are optimized according to temperature-induced effects when the force-constant tensor in Eq. 1 is fitted to AIMD forces and displacements.

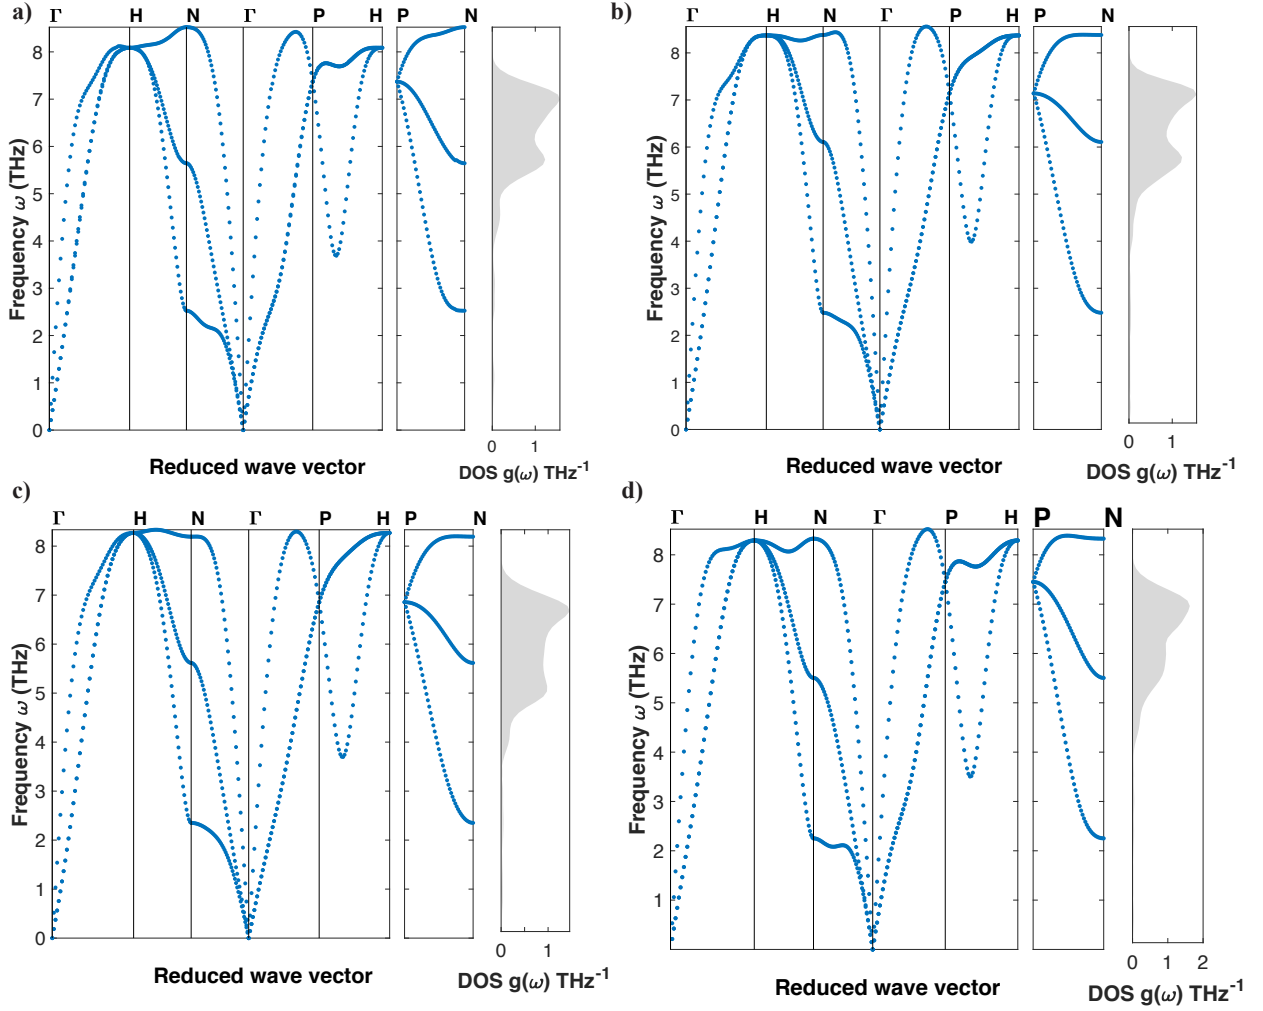

FIG. S2. a) The anharmonic phonon dispersion and density of states for the bulk bcc Ti at a) 1300 K, b) 1400 K, c) 1500 K and d) 1600 K, obtained from the TDEP method.

## SII. CALCULATION OF VACANCY FORMATION ENTHALPY

Since the bcc phase of IIIB and IVB metals is a high-temperature phase, the total DFT energy at zero temperature is not a good approximation for the enthalpy of the system, while it is usually used for mechanically stable phases. We obtain the enthalpy of the bulk or defected bcc phase as the following

$$H = \langle U \rangle + \langle p \rangle V, \quad (4)$$

where  $\langle U \rangle$  is the NVT ensemble average of the internal energy, consisting of the potential and kinetic energy at each temperature,  $\langle p \rangle$  is the average pressure, and  $V$  is the total volume of the system. The canonical ensemble averages are obtained by block averaging of AIMD internal energy and pressure according to the scheme described in appendix D.3 of Ref. [12]. To ensure that the energy and pressure values are obtained from uncorrelated MD snapshots, the characteristic decay time of the MD trajectory is obtained from the limit of the following product function,  $P(t_B)$ , when  $t_B \rightarrow \infty$  [12].

$$P(t_B) = t_B \times \frac{\sigma^2(\bar{A}_B)}{\langle A^2 \rangle - \langle A \rangle^2} \quad (5)$$

Here,  $\bar{A}_B$  is the block average of any observable  $A$  (i.e., the time average over a finite time  $t_B$ ),  $\sigma^2$  is the variance of the block average, and  $\langle A \rangle$  is the ensemble average of  $A$ . In the limit of block time being much larger than the characteristic decay time of the observable time correlation function,  $P$  will approach the characteristic decay time (refer to Ref. [12] for more details). Fig. S3(b) shows the  $P(t_B)$  function as a function of block time, obtained by time averaging the internal energy  $U$  from the AIMD trajectory. For a block time larger than 0.2 ps, the  $P$  value does not change dramatically and merely oscillates around 0.015 ps, which is the characteristic decay time of the AIMD time correlation function. As shown in Fig. S3(a), the time required for the Nose-Hoover thermostat to equilibrate is determined to be 1 ps according to the temperature-time curve. The average internal energy and pressure for each system at each temperature are obtained by averaging the AIMD snapshots internal energy and pressure captured every 0.1 ps (larger than the decay time) after the burning equilibration time, as shown in Fig. S3(c-d). The vacancy formation enthalpy is then calculated as

$$\Delta H_v = H^{tot}(N-1) - \frac{N-1}{N} H^{tot}(N), \quad (6)$$

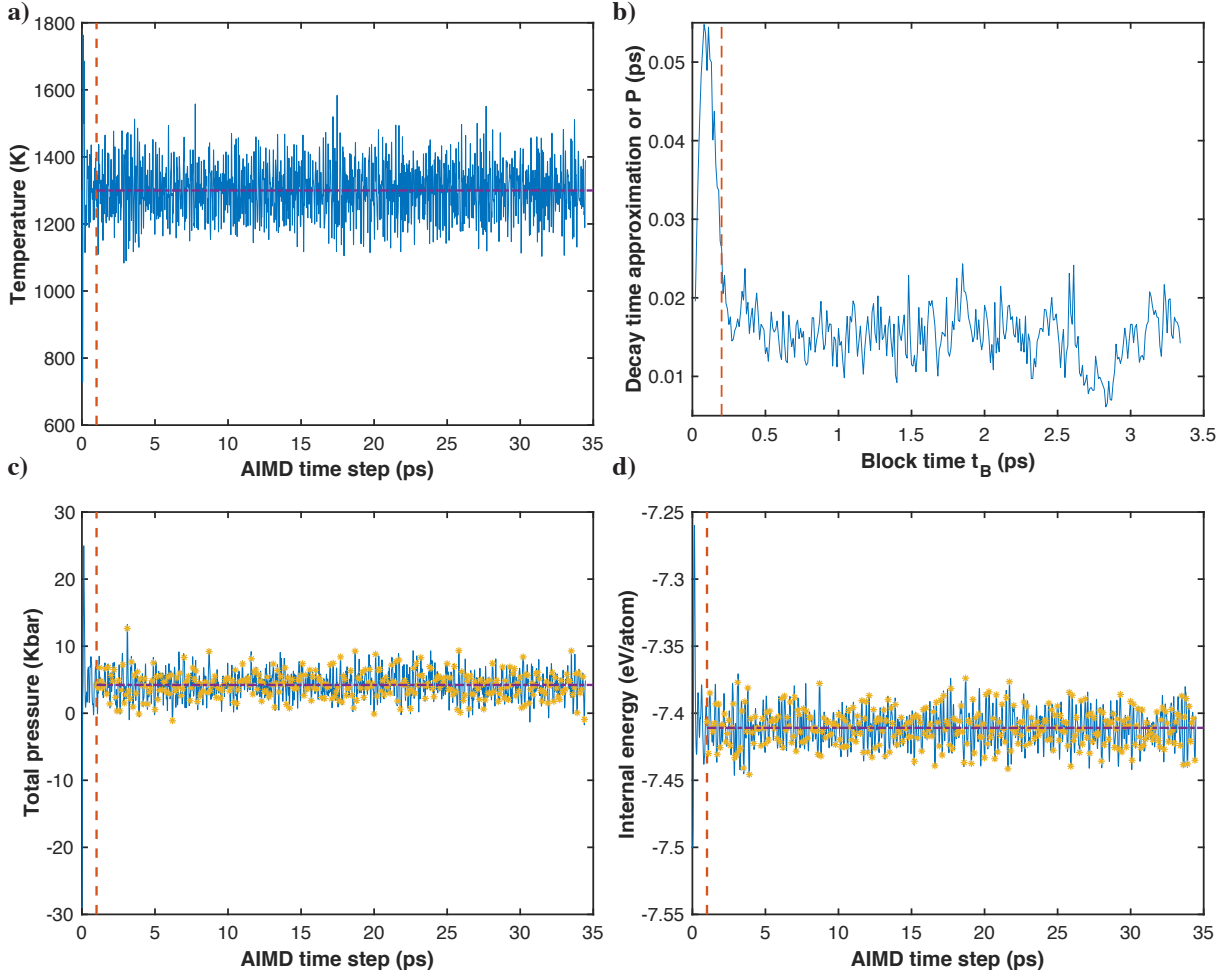

FIG. S3. a) Temperature vs. time for the canonical molecular dynamics simulation of bulk bcc Ti at 1300 K using the Nose–Hoover thermostat. The thermalization time (a.k.a. the burning time) is illustrated by the dashed line. b) The P value,  $t_B \times \frac{\sigma^2(\bar{U}_B)}{\langle U^2 \rangle - \langle U \rangle^2}$ , for the MD trajectory as a function of the block time,  $t_B$ . For a block time larger than 0.2 ps (dashed line), the P value does not change and merely oscillates around 0.015 ps, which is the characteristic decay time. c-d) The AIMD pressure and internal energy vs. time. The star marks indicate the values captured for statistical averaging and the dotted lines are the mean values.

where  $H^{tot}(N-1)$  and  $H^{tot}(N)$  are the enthalpy for the bulk and defected systems, respectively. A correction term is added to the vacancy formation enthalpy as described in the next section.

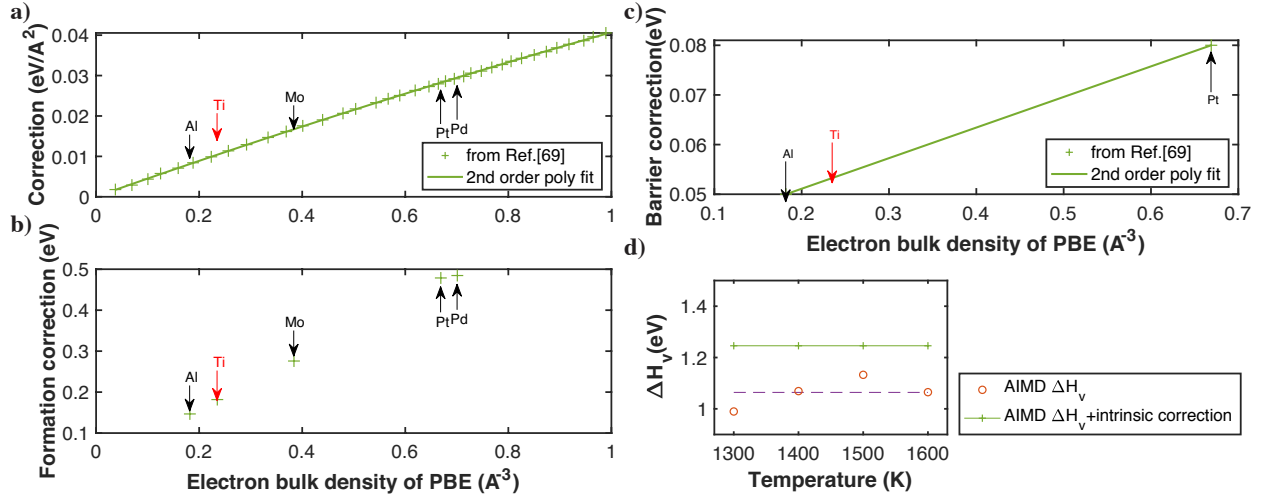

FIG. S4. a) The intrinsic surface correction term per area as a function of bulk valence electron density of the PBE exchange-correlation functional. Cross values are extracted from Fig. 5 of Ref. [13]. b) The total correction term for vacancy formation energy for Ti, Al, Mo, Pt, and Pd. c) The total correction term for vacancy migration energy for Ti, Al and Pt. d) The vacancy formation enthalpy in bcc Ti as a function of temperature. The circles are the statical average formation enthalpy obtained from AIMD simulation using the PBE exchange-correlation functional. The crosses are the formation enthalpy values including the explicit intrinsic surface correction term.

### SIII. CALCULATION OF INTRINSIC SURFACE CORRECTION TERM FOR THE VACANCY FORMATION AND MIGRATION ENTHALPIES

It has been shown in the literature that density functional theory underestimates the vacancy formation and migration enthalpies [13–18]. This underestimation has been associated to electron correlation effects near electronic edges of the intrinsic surface which is formed due to vacancy formation [14], and is predominantly a function of bulk electron density for both the LDA and GGA exchange-correlation functional formalism [13]. Fig. S4(a) illustrates the explicit correction term per area as a function of the bulk electron density for the PBE exchange-correlation functional [19] extracted from Fig.5 of Ref. [13]. We used the PBE exchange-correlation functional as implemented in PAW-PBE pseudopotential of VASP [20]. The number of valence electrons for each conventional bcc unit cell is  $2N_{elect} = 2 \times 4$  and the bulk electron density is  $\rho = \frac{2N_{elect}}{a_0^3} = 0.235 \text{ \AA}^{-3}$ , where  $a_0 = 3.24$ . We calculated the exposed surface area of vacancy in bcc Ti to be  $17.46 \text{ \AA}^2$ , based on the vacancy radius in

fcc Al and the scaling scheme described in table III of Ref. [13]. Fig. S4(b) illustrate the vacancy formation correction term for bcc Ti alongside the correction values for Al, Mo, Pt, and Pd [13]. We calculate the final correction term by multiplying the correction term per area in Fig. S4(a) by the exposed vacancy surface in each element, which is in good agreement with values presented in table III of Ref. [13]. The migration barrier energy is calculated more accurately than the formation energy in DFT, simply because two more similar energies are compared (i.e., propagation of surface formation error along the transition path) than when calculating the formation energy [13]. As illustrated in Fig. S4(c), we calculated the explicit correction term for migration energy by interpolating the results for fcc Al and fcc Pt extracted from Ref. [14] and Ref. [13], respectively. Fig. S4(d) indicates the AIMD formation enthalpy and the final formation enthalpy which includes the intrinsic surface correction term.

#### SIV. CALCULATION OF VACANCY FORMATION ENTROPY AND EQUILIBRIUM MONOVACANCY CONCENTRATION

The vacancy formation entropy is calculated at each temperature according to the following equation:

$$\Delta S_v = S^{tot}(N-1) - \frac{N-1}{N} S^{tot}(N), \quad (7)$$

where  $N$  is the number of atoms in the supercell and  $S^{tot}(N-1)$  and  $S^{tot}(N)$  are the vibrational entropy for bcc with a monovacancy and bulk bcc, respectively. The vibrational entropy is calculated given the anharmonic and temperature-dependent phonon frequencies and density of states according to the following equation:

$$S_{vib} = -k_B \int_0^\infty \ln \left[ 2 \sinh\left(\frac{\hbar\omega(T)}{2k_B T}\right) \right] g(\omega(T)) d\omega, \quad (8)$$

where  $\omega(T)$  and  $g(\omega(T))$  are temperature-dependent phonon frequencies and density of states, respectively. The vacancy formation entropy for bcc Ti at each temperature is shown in Fig.4(b) in the main text and for bcc Zr is shown in Fig. S11. The equilibrium monovacancy concentration,  $C_v$ , is calculated according to

$$C_v = \exp\left(-\frac{\Delta H_v}{k_B T}\right) \exp\left(\frac{\Delta S_v}{k_B}\right), \quad (9)$$

where  $\Delta H_v$  and  $\Delta S_v$  are enthalpy and entropy of monovacancy formation, respectively. The monovacancy concentration for bcc Ti obtained according to the anharmonic phonon

analysis is presented in Fig. 4 in the main text (similar plot for bcc Zr is presented in Fig. S11). We also calculate the vacancy formation entropy and concentration for the case where the harmonic phonon analysis is used (and existing imaginary phonon frequencies are ignored). As illustrated in Fig. 4 of the main text and Fig. S11, in the harmonic approximation the formation entropy is independent of temperature, since it is obtained based on temperature-independent phonon frequencies and DOS at 0 K.

## SV. CALCULATION OF DIFFUSION COEFFICIENT FOR BCC ZIRCONIUM

To confirm the validity of the proposed approach, we calculate the diffusion coefficient for bcc Zr in addition to bcc Ti. In the following, we elaborate on diffusivity calculation for bcc Zr, which is conducted in the same way as bcc Ti explained in the main letter. Fig S5 illustrates the zero-temperature phonon dispersion, density of states, and total energy for a  $6 \times 6 \times 6$  supercell of bcc Zr with a monovacancy (the lattice parameter is  $a_0 = 3.59 \text{ \AA}$ ). The dispersion and DOS are obtained from DFT forces and displacements according to the finite displacement approach implemented in the Vienna Ab-initio Simulation Package (VASP) [20–23]. The projector augmented wave (PAW) method [24, 25] with energy cutoff of 229.9 eV and the generalized gradient approximation (GGA) [20, 23, 26] with the PBE [19] exchange-correlation are used. The pseudo-potential includes 12 electrons in the valance shell (the Zr\_sv as implemented in VASP). As shown in Fig. S6, the converged temperature-dependent phonon dispersion for bcc Zr is obtained at the range of 1300 K to 1700 K according to the SCAILD method explained in section SI. The effective vibration frequency along the vacancy diffusive path,  $\nu^*$ , is assumed to be the frequency of the  $2/3L \langle 111 \rangle$  phonon mode, as shown by the star mark in Fig. S6(d). Fig. S7 indicates the T-dependent phonon dispersions for both the bulk bcc zirconium and the bcc Zr including a vacancy obtained by the TDEP method as explained in section SI. The AIMD forces and displacement are captured every 0.02 ps in a trajectory of 35 ps, after thermalization of the system for 1 ps (for details on the burning and decay time Fig. S8). The vacancy formation enthalpy is obtained according to Eq. 6, where the enthalpy for the bulk and defected systems are obtained from AIMD energy and pressure averages according to Eq. 4. For statistical averaging, we capture AIMD energy and pressure every 0.1 ps (above the 0.02 ps decay time shown in Fig S8(d)) and after the 1 ps thermalization time as shown in Fig S8(a). The vacancy formation

enthalpy from average AIMD calculation is explicitly corrected for the “intrinsic surface” error of DFT, as explained in section [SIII](#). Moreover, the migration enthalpy is approximated as the DFT energy difference of the initial and transition states, as illustrated in Fig [S5](#)(c-d). The migration energy is also corrected for the internal surface effect according to details of section [SIII](#). Fig. [S9](#) indicates the correction terms and corrected vacancy formation enthalpy for bcc Zr.

Fig. [S10](#) indicates the T-dependent phonon density of states for the bulk and defected bcc Zr, obtained by the TDEP method. The vibrational entropy for each system is obtained according to Eq. [8](#) and the vacancy formation entropy is then obtained according to Eq. [7](#). Fig. [S11](#) shows the formation entropy and equilibrium concentration for a monovacancy in bcc Zr obtained according to the anharmonic vibrational analysis. It is compared with the results obtained by a standard harmonic treatment of lattice vibration as explained in section [SIV](#).

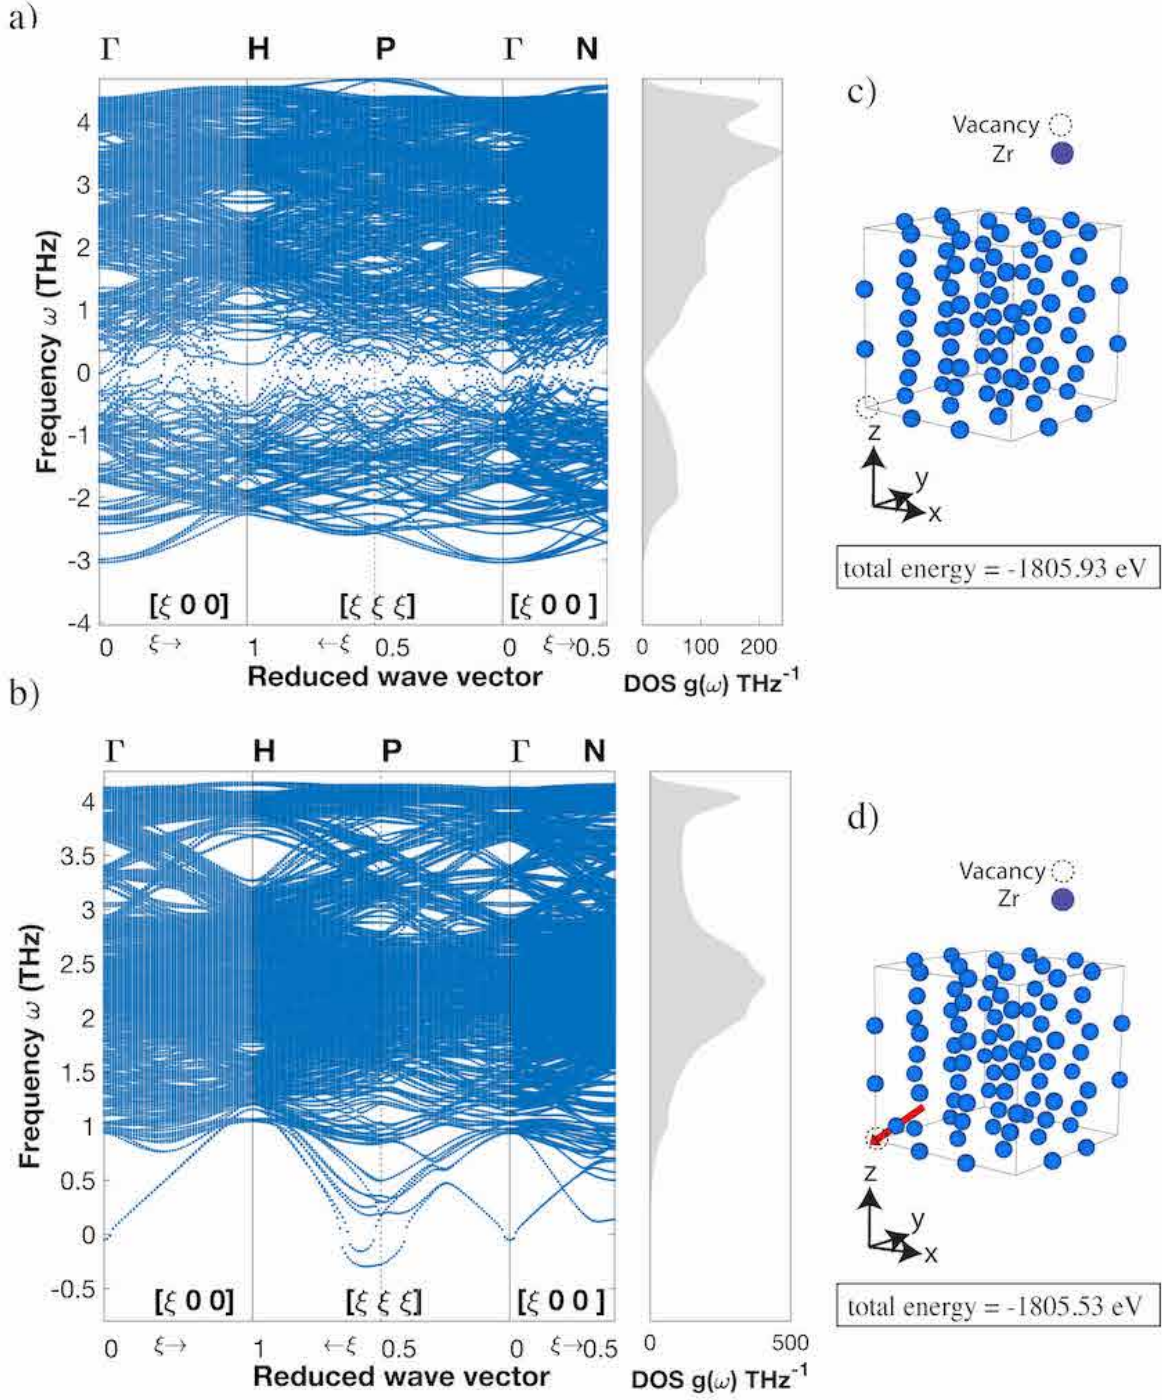

FIG. S5. DFT harmonic phonon dispersion and density of states (DOS) for a  $6 \times 6 \times 6$  supercell of bcc zirconium including 215 atoms and a monovacancy a) at the bcc site, and b) migrated half way to the nearest neighbor bcc site along  $[111]$  direction. Phonon instabilities are depicted as negative frequencies in the dispersion curves. The atomic configuration for the initial and intermediate states of vacancy diffusion are illustrated in c) and d), respectively. A conventional supercell is presented for visualization simplicity.

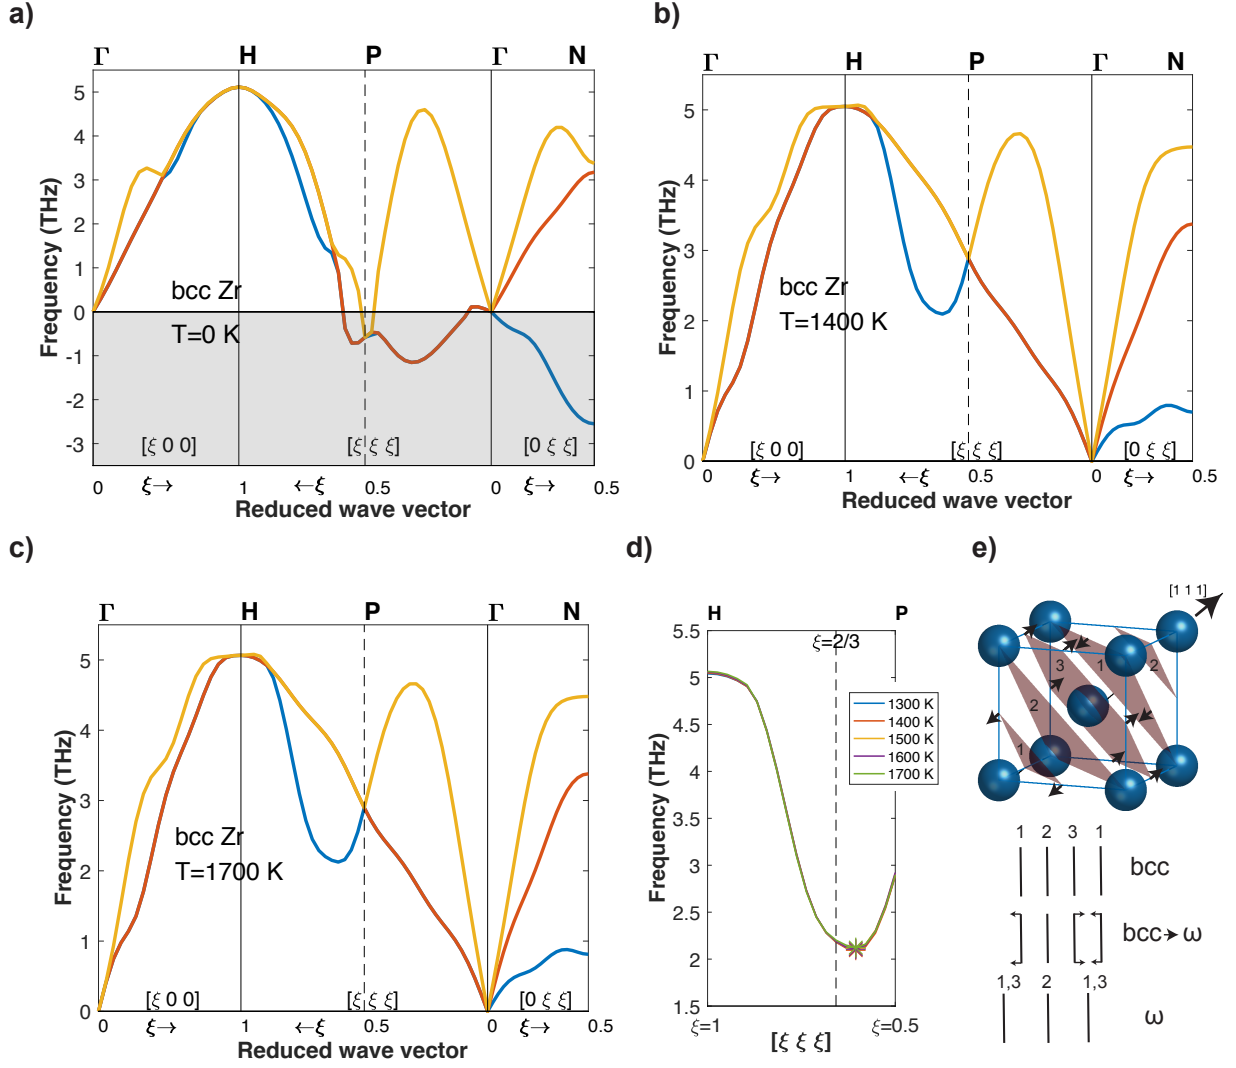

FIG. S6. Phonon dispersion for a bulk defect-free  $6 \times 6 \times 6$  supercell of bcc zirconium including 216 atoms at a) 0 K, b) 1400 K, and c) 1700 K. d) The longitudinal phonon branch along the  $[\xi\xi\xi]$  reduced wave vector (between H and P high-symmetry points) from 1300 K to 1700 K. The star marks in (d) represent the negative dip on the phonon branch. e) The trigonal distortion of (111) atomic planes along the  $[111]$  direction associated with the eigenvector of  $\xi = \frac{2}{3}$  phonon mode along the  $\Gamma$ -P-H branch. A complete collapse of atomic planes 1 and 3 results in the hexagonal  $\omega$  phase.

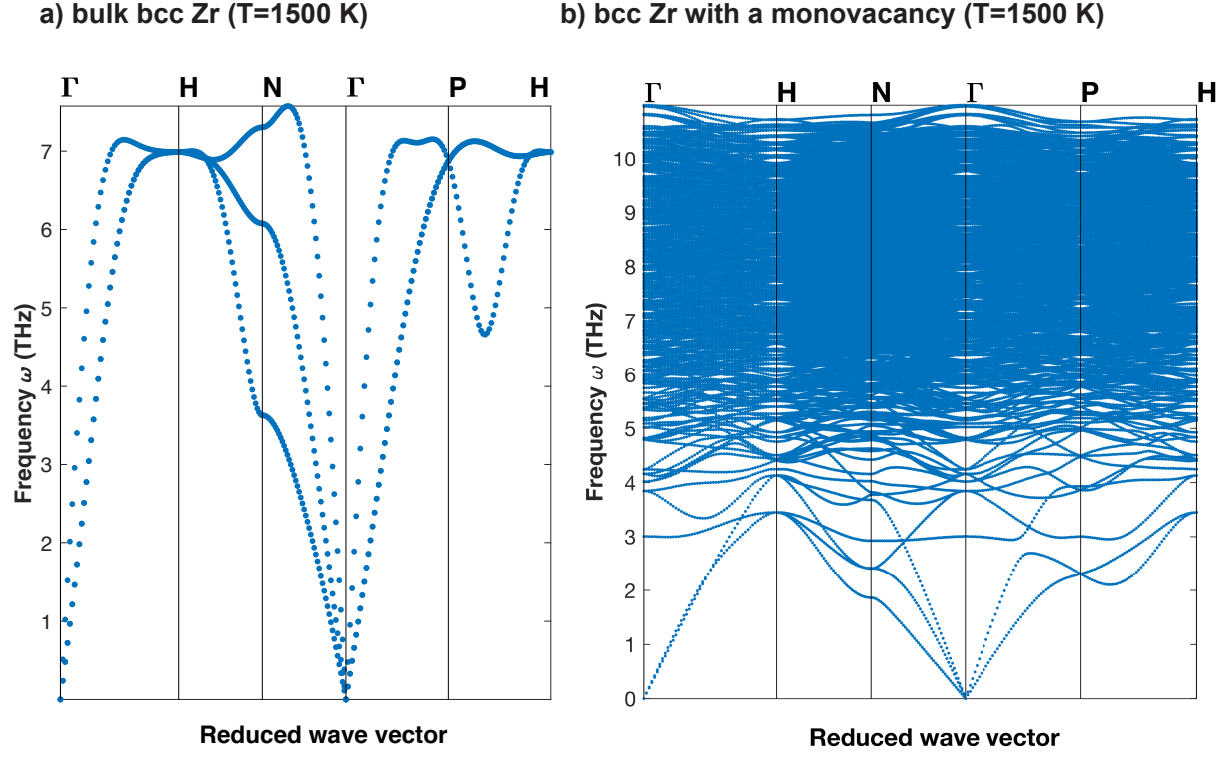

FIG. S7. The anharmonic phonon dispersion for a) a  $6 \times 6 \times 6$  supercell of bcc zirconium including 216 atoms and b) bcc Zr with a monovacancy including 215 atoms at 1500 K. The phonon dispersion and DOS for the defected system are obtained by enforcing the bcc crystal symmetry.

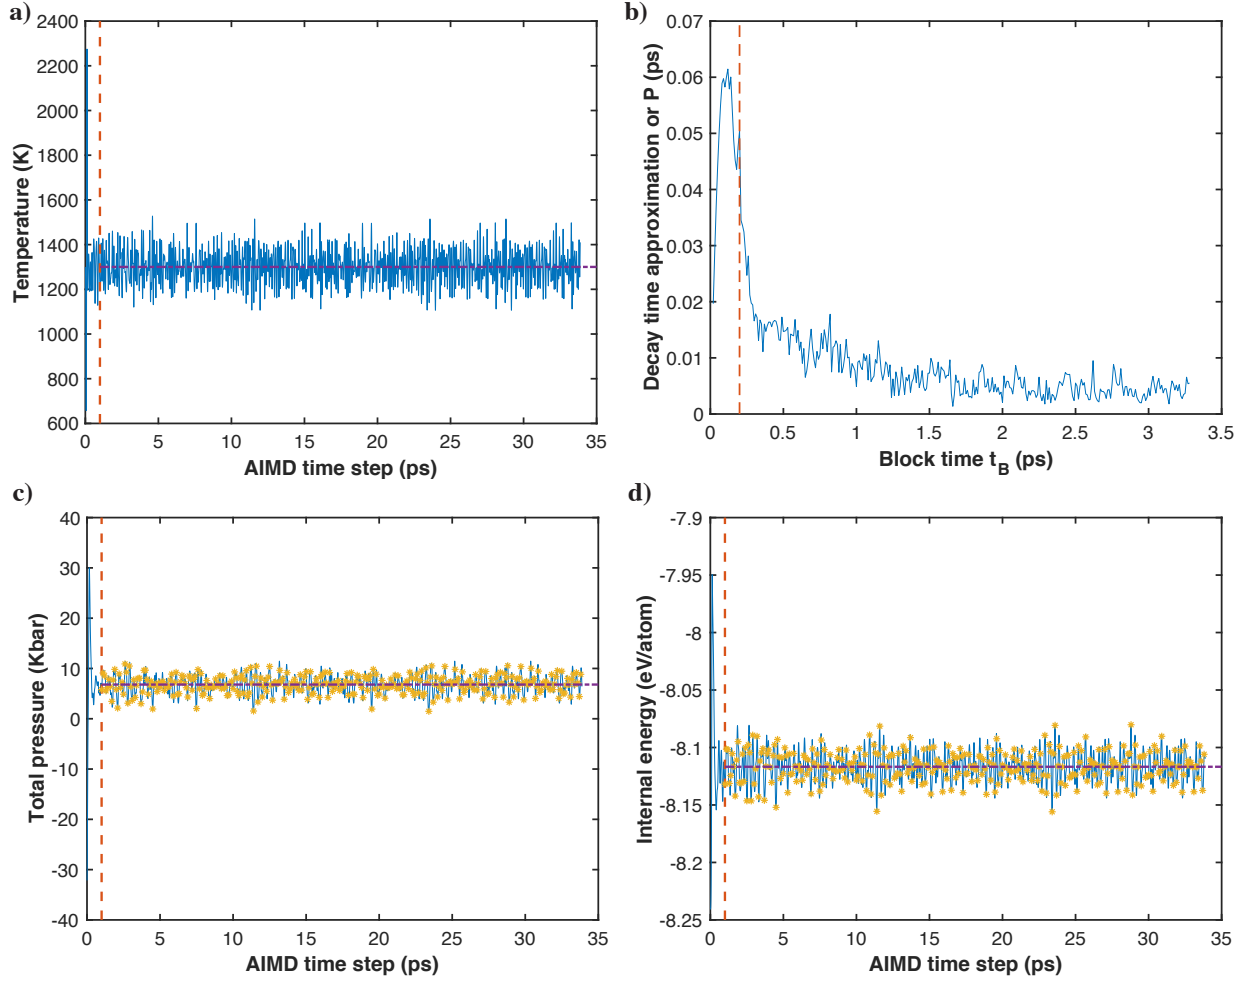

FIG. S8. a) Temperature vs. time for the canonical molecular dynamics simulation of bulk bcc Zr at 1300 K using the Nose–Hoover thermostat. The thermalization time (a.k.a. the burning time) is illustrated by the dashed line. b) The P value,  $t_B \times \frac{\sigma^2(\bar{U}_B)}{\langle U^2 \rangle - \langle U \rangle^2}$ , for the MD trajectory as a function of the block time,  $t_B$ . For a block time larger than 0.2 ps (dashed line), the P value does not change and merely oscillates around 0.005 ps, which is the characteristic decay time. c-d) The AIMD pressure and internal energy vs. time. The star marks indicate the values captured for statistical averaging.

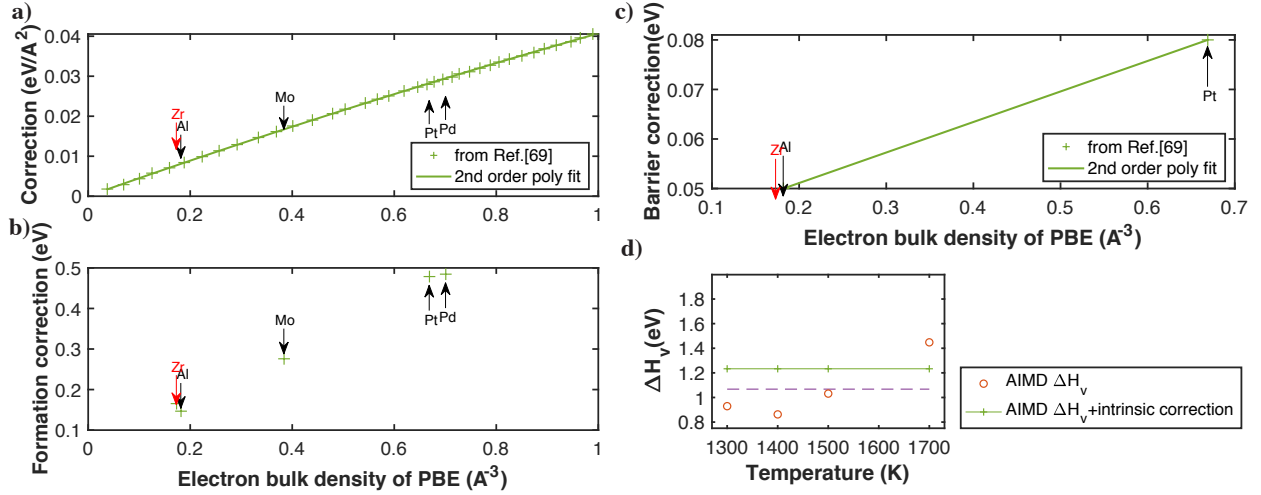

FIG. S9. a) The intrinsic surface correction term per area as a function of bulk valence electron density of the PBE exchange-correlation functional. Cross values are extracted from Fig. 5 of Ref. [13]. b) The total correction term for vacancy formation energy for Zr, Al, Mo, Pt, and Pd. c) The total correction term for vacancy migration energy for Zr, Al and Pt. d) The vacancy formation enthalpy in bcc Zr as a function of temperature. The circles are the static average formation enthalpy obtained from AIMD simulation using the PBE exchange-correlation functional. The crosses are the formation enthalpy values including the explicit intrinsic surface correction term.

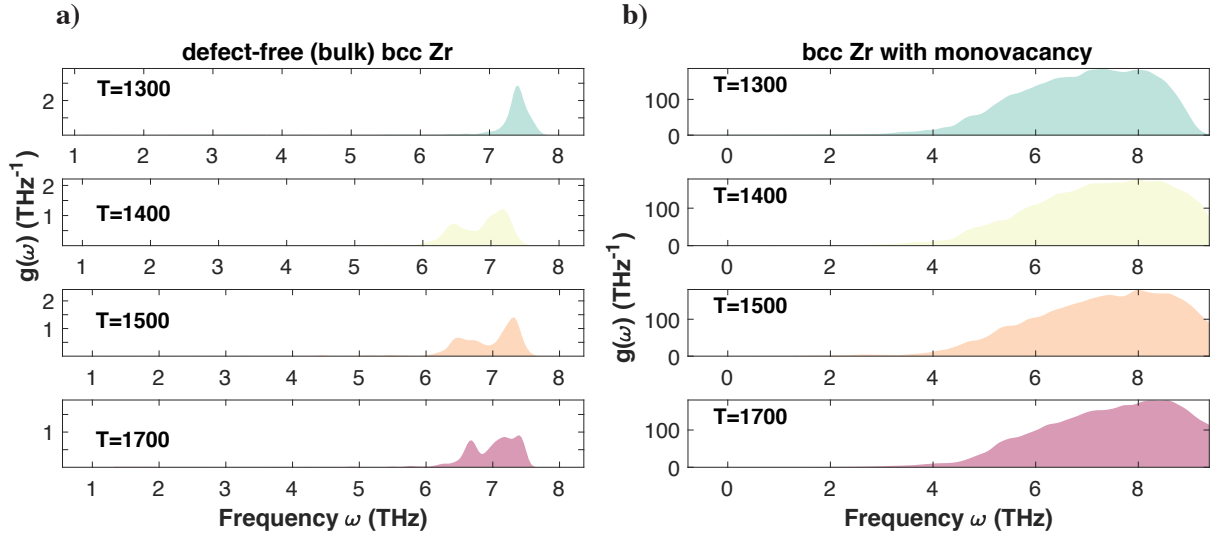

FIG. S10. The anharmonic phonon density of states for bulk bcc Zr (the left plots) and the bcc phase with a monovacancy (the right plots) at different temperatures.

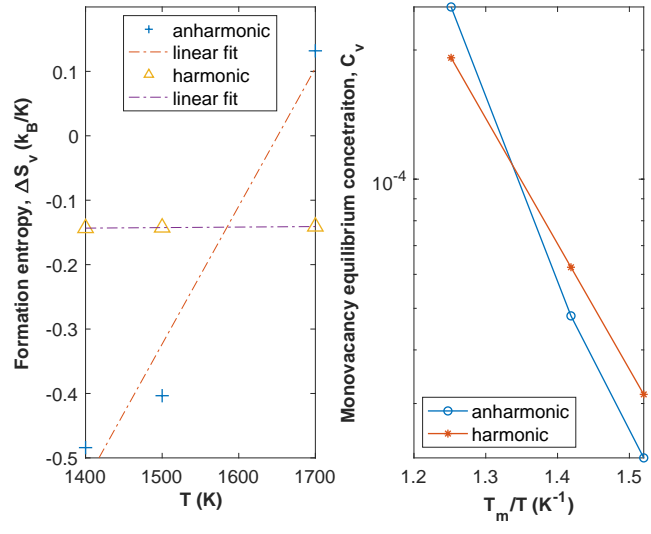

FIG. S11. The formation entropy and equilibrium concentration versus temperature for monovacancy in bcc Zr.  $T_m=2153$  K.

- 
- [1] N. R. Werthamer, “Self-Consistent Phonon Formulation of Anharmonic Lattice Dynamics,” [Physical Review B](#) **1**, 572–581 (1970).
- [2] P. Souvatzis, O. Eriksson, M. I. Katsnelson, and S. P. Rudin, “Entropy Driven Stabilization of Energetically Unstable Crystal Structures Explained from First Principles Theory,” [Physical Review Letters](#) **100**, 095901 (2008).
- [3] P. Souvatzis, O. Eriksson, M.I. Katsnelson, and S.P. Rudin, “The self-consistent ab initio lattice dynamical method,” [Computational Materials Science](#) **44**, 888 – 894 (2009).
- [4] O. Hellman, I. A. Abrikosov, and S. I. Simak, “Lattice dynamics of anharmonic solids from first principles,” [Physical Review B](#) **84**, 180301(R) (2011).
- [5] Olle Hellman, Peter Steneteg, I. A. Abrikosov, and S. I. Simak, “Temperature dependent effective potential method for accurate free energy calculations of solids,” [Physical Review B](#) **87**, 104111 (2013).
- [6] William G. Hoover and Brad Lee Holian, “Kinetic moments method for the canonical ensemble distribution,” [Physics Letters A](#) **211**, 253 – 257 (1996).
- [7] S. Nosé, “A molecular dynamics method for simulations in the canonical ensemble,” [Molecular Physics](#) **52**, 255–268 (1984).
- [8] Shuichi Nosé, “A unified formulation of the constant temperature molecular dynamics methods,” [The Journal of Chemical Physics](#) **81**, 511–519 (1984).
- [9] William G. Hoover, “Canonical dynamics: Equilibrium phase-space distributions,” [Phys. Rev. A](#) **31**, 1695 (1985).
- [10] Glenn J. Martyna, Michael L. Klein, and Mark Tuckerman, “Nosé-Hoover chains: The canonical ensemble via continuous dynamics,” [The Journal of Chemical Physics](#) **97**, 2635–2643 (1992).
- [11] A Togo and I Tanaka, “First principles phonon calculations in materials science,” [Scr. Mater.](#) **108**, 1–5 (2015).
- [12] “Appendix d - statistical errors,” in [Understanding Molecular Simulation \(Second Edition\)](#), edited by Daan Frenkel and Berend Smit (Academic Press, San Diego, 2002) second edition ed., pp. 525 – 532.
- [13] Thomas R. Mattsson and Ann E. Mattsson, “Calculating the vacancy formation energy in

- metals: Pt, pd, and mo,” [Phys. Rev. B \*\*66\*\*, 214110 \(2002\)](#).
- [14] Karin Carling, Göran Wahnström, Thomas R. Mattsson, Ann E. Mattsson, Nils Sandberg, and Göran Grimvall, “Vacancies in metals: From first-principles calculations to experimental data,” [Phys. Rev. Lett. \*\*85\*\*, 3862–3865 \(2000\)](#).
  - [15] Christoph Freysoldt, Blazej Grabowski, Tilmann Hickel, Jörg Neugebauer, Georg Kresse, Anderson Janotti, and Chris G. Van de Walle, “First-principles calculations for point defects in solids,” [Rev. Mod. Phys. \*\*86\*\*, 253–305 \(2014\)](#).
  - [16] R. Nazarov, T. Hickel, and J. Neugebauer, “Vacancy formation energies in fcc metals: Influence of exchange-correlation functionals and correction schemes,” [Phys. Rev. B \*\*85\*\*, 144118 \(2012\)](#).
  - [17] Ann E. Mattsson, Ryan R. Wixom, and Rickard Armiento, “Electronic surface error in the Si interstitial formation energy,” [Phys. Rev. B \*\*77\*\*, 155211 \(2008\)](#).
  - [18] Ann E. Mattsson, Rickard Armiento, Peter A. Schultz, and Thomas R. Mattsson, “Nonequivalence of the generalized gradient approximations PBE and PW91,” [Phys. Rev. B \*\*73\*\*, 195123 \(2006\)](#).
  - [19] J. P. Perdew, K. Burke, and M. Ernzerhof, “Generalized gradient approximation made simple,” [Phys. Rev. Lett. \*\*77\*\*, 3865–3868 \(1996\)](#).
  - [20] G. Kresse and D. Joubert, “From ultrasoft pseudopotentials to the projector augmented-wave method,” [Phys. Rev. B \*\*59\*\*, 1758–1775 \(1999\)](#).
  - [21] G. Kresse and J. Hafner, “Ab initio molecular dynamics for liquid metals,” [Phys. Rev. B \*\*47\*\*, 558–561 \(1993\)](#).
  - [22] G. Kresse and J. Furthmüller, “Efficiency of ab-initio total energy calculations for metals and semiconductors using a plane-wave basis set,” [Computational Materials Science \*\*6\*\*, 15 – 50 \(1996\)](#).
  - [23] G. Kresse and J. Furthmüller, “Efficient iterative schemes for ab initio total-energy calculations using a plane-wave basis set,” [Phys. Rev. B \*\*54\*\*, 11169–11186 \(1996\)](#).
  - [24] P. E. Blöchl, “Projector augmented-wave method,” [Phys. Rev. B \*\*50\*\*, 17953–17979 \(1994\)](#).
  - [25] G. Kresse and D. Joubert, “From ultrasoft pseudopotentials to the projector augmented-wave method,” [Phys. Rev. B \*\*59\*\*, 1758–1775 \(1999\)](#).
  - [26] John P. Perdew, “Generalized gradient approximation for the fermion kinetic energy as a functional of the density,” [Physics Letters A \*\*165\*\*, 79 – 82 \(1992\)](#).
